# Supplementary material for: VisCoder: Fine-Tuning LLMs for Executable Python Visualization Code Generation
Source: arXiv:2506.03930 source file (2025-09-29)
Supplement: Supplementary file 1 [file check_list.tex]

\newpage
\clearpage

\section{Ethics and Reproducibility Statements}

\subsection{Potential Risks}
This work focuses on training and evaluating large language models to generate Python visualization code. While outputs are validated for executability, there remains a potential risk of generating misleading or malformed plots, particularly in cases of silent failures. No personal, sensitive, or user-generated content is involved.

\subsection{Discuss the License for Artifacts}
All released artifacts are provided under permissive licenses suitable for academic research. License terms permit use, modification, and redistribution in accordance with each license’s conditions.

\subsection{Artifact Use Consistent With Intended Use}
All external datasets and software components were used in accordance with their original license agreements and intended purposes. Derived artifacts are intended solely for research and educational use, and are not authorized for commercial deployment or redistribution.

\subsection{Data Contains Personally Identifying Info or Offensive Content}
All data was either synthetically generated or obtained from public sources. Automated filters and manual review were applied to ensure that no samples contain personally identifying information or offensive content. All instructions and tables are free of references to real individuals, groups, or sensitive contexts.

\subsection{Documentation of Artifacts}
All released artifacts are accompanied by documentation describing their structure, content format, intended use, and evaluation methodology. Sufficient metadata and usage instructions are provided to support inspection, reproduction, and downstream research use.

\subsection{Parameters for Packages}
All external packages used during training and evaluation were applied in accordance with standard practices. Default parameters were used unless otherwise specified. Any deviations from default settings are documented in the accompanying implementation materials.

\subsection{AI Assistants in Research or Writing}
Used ChatGPT to capture grammar errors in the manuscript.
